# Supplementary material for: Astronomy's climate emissions: Global travel to scientific meetings in 2019
Source: arXiv:2405.00104 source file (2024-04-30)
Supplement: Supplementary file 1 [file Supplementary_Material_Astronomys_Climate_Emissions.pdf]

# Astronomy's climate emissions: global travel to scientific meetings in 2019 – Supplementary Material

Andrea Gokus,<sup>1,2,3\*</sup> Knud Jahnke,<sup>4</sup> Paul M. Woods,<sup>5</sup> Vanessa A. Moss,<sup>6,7</sup>  
 Volker Ossenkopf-Okada,<sup>8</sup> Elena Sacchi,<sup>9</sup> Adam R. H. Stevens,<sup>10</sup>  
 Leonard Burtscher,<sup>11</sup> Cenk Kayhan,<sup>12</sup> Hannah Dalglish,<sup>13,14</sup> Victoria Grinberg,<sup>15</sup>  
 Travis A. Rector,<sup>16</sup> Jan Rybizki,<sup>17</sup> and Jacob White<sup>18</sup>

<sup>1</sup>Department of Physics & McDonnell Center for the Space Sciences,  
 Washington University in St. Louis, One Brookings Drive, St. Louis, MO 63130, USA

<sup>2</sup>Dr. Karl Remeis Sternwarte & ECAP,  
 Universität Erlangen-Nürnberg, Sternwartstr. 7, 96049 Bamberg, Germany

<sup>3</sup>Institut für Theoretische Physik und Astrophysik,  
 Universität Würzburg, Emil-Fischer-Straße 31, 97074 Würzburg, Germany

<sup>4</sup>Max-Planck-Institut für Astronomie, Königstuhl 17, 69117 Heidelberg, Germany

<sup>5</sup>Independent researcher, London, UK

<sup>6</sup>ATNF, CSIRO Space and Astronomy, PO Box 76, Epping, NSW 1710, Australia

<sup>7</sup>Sydney Institute for Astronomy, School of Physics A28, University of Sydney, NSW 2006, Australia

<sup>8</sup>Universität zu Köln, I. Physikalisches Institut, Zùlpicher Str. 77, 50937 Köln, Germany

<sup>9</sup>Leibniz-Institut für Astrophysik Potsdam (AIP), An der Sternwarte 16, 14482 Potsdam, Germany

<sup>10</sup>International Centre for Radio Astronomy Research,  
 The University of Western Australia, Crawley, WA 6009, Australia

<sup>11</sup>Leiden Observatory, PO Box 9513, 2300 RA, Leiden, The Netherlands

<sup>12</sup>Department of Astronomy and Space Sciences,  
 Faculty of Science, Erciyes University, 38030 Melikgazi, Kayseri, Türkiye

<sup>13</sup>Department of Physics, University of Oxford, Keble Rd, Oxford, OX1 3RH, UK

<sup>14</sup>Politics & International Relations, University of Southampton, University Rd, Southampton, SO17 1BJ, UK

<sup>15</sup>European Space Agency (ESA), European Space Research and Technology Centre (ESTEC)  
 Keplerlaan 1, 2201 AZ Noordwijk, The Netherlands

<sup>16</sup>University of Alaska Anchorage, 3211 Providence Dr., Anchorage, AK, 99508 USA

<sup>17</sup>Weimar Institute of Applied Construction Research, Über der Nonnenwiese 1, 99428 Weimar, Germany

<sup>18</sup>Independent researcher, Vancouver, Canada

\*To whom correspondence should be addressed; E-mail: gokus@wustl.edu / dr.andrea.gokus@gmail.com

## Hotel CO<sub>2</sub>e emissions

In-person conferences require travel to the conference venue, and also — if not at a local venue — hotel accommodation. Staying at a hotel comes with its own environmental footprint, due to electricity consumption, heating and cooling, catering, as well as waste and wastewater disposal needs. To assess

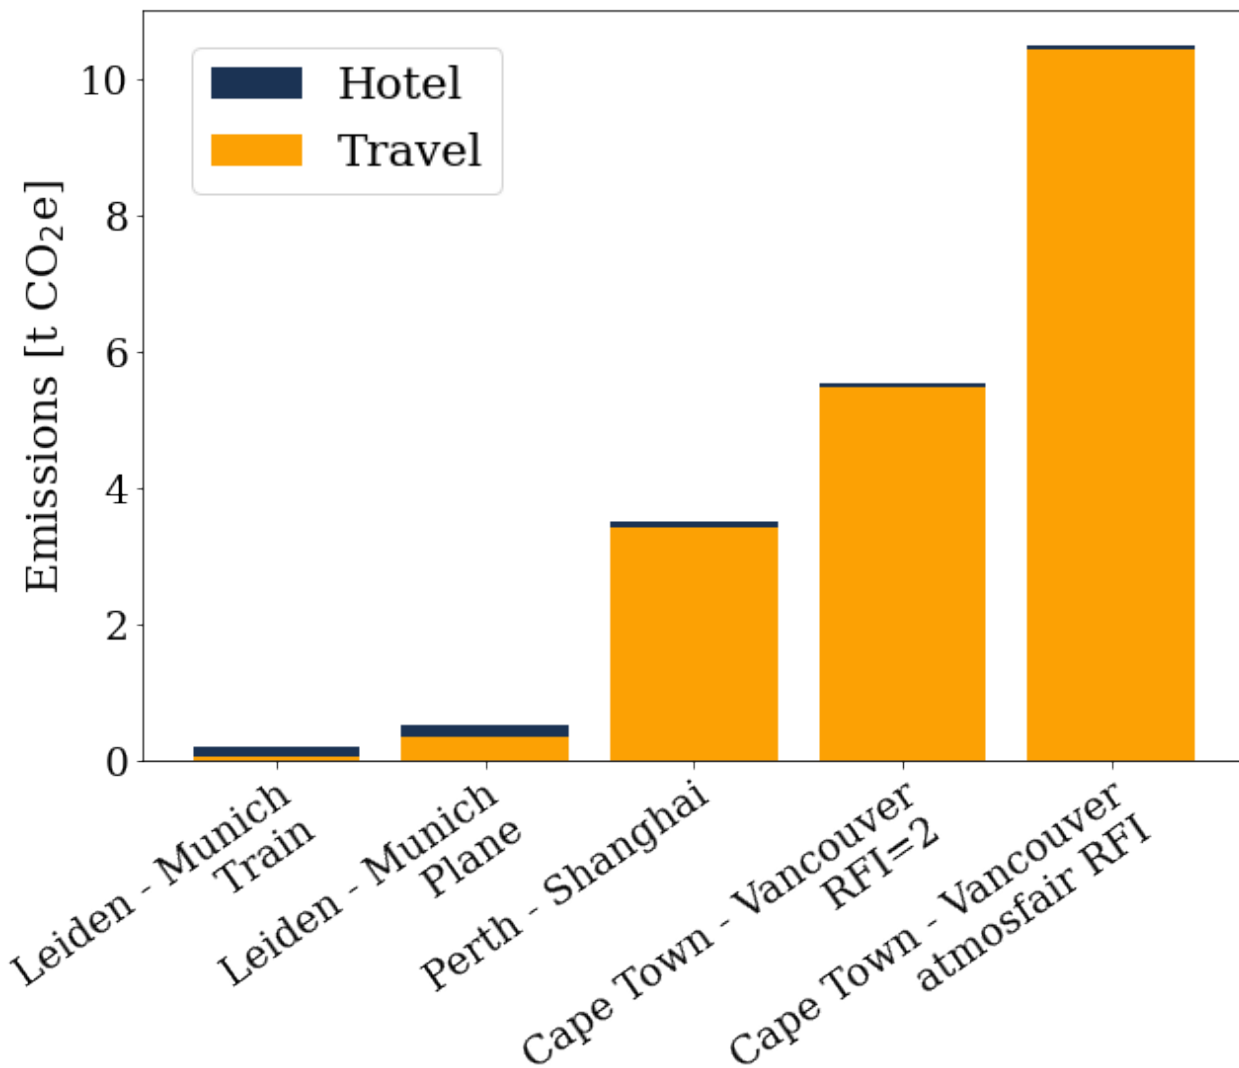

**Supplementary Figure 1:** Emissions for travel and hotel accommodation for three exemplary trips, each with a stay of six nights at a hotel. The contributions to the overall emissions are from travel (yellow) and accommodation (blue). To first order, flight emissions scale with distance. Train travel produces substantially lower GHG emissions than flying, and, except for longer stays in combination with train travel, the contribution by hotel accommodation is a minor fraction of total emissions. For each trip, the contribution from hotel- and travel-related emissions are, respectively: 71.6% / 28.4% (Leiden - Munich by train); 29.8% / 70.2% (Leiden - Munich by plane); 2.7% / 97.3% (Perth - Shanghai); 1.0% / 99.0% (Cape Town - Vancouver with RFI=2); 0.5 % / 99.5%(Cape Town - Vancouver with atmosfair RFI value). When comparing the impact of GHG emissions, the assumed radiative forcing index (RFI) for flights is important, as well assumptions on flight route length vs. great circles, and, potentially, the type of aircrafts. An RFI value of 1.95, as assumed throughout this study, is on the lower end of potential impact factors. Flight emission calculations through the atmosfair.de website are taking into account a higher RFI as well as typical aircraft types and real-world flight routes, which can result in substantially higher emission values.

the relative GHG emissions of accommodation versus travel we used data provided to us by atmosfair, who created and maintain emission calculation standards not only for means of travel, but also hotels<sup>1</sup>. A typical hotel stay can emit from below 5 kgCO<sub>2</sub> per night for a standard single room of a 1- or 2-star hotel to beyond 40 kgCO<sub>2</sub> in a 4- or 5-star hotel. The emission will vary strongly between countries with low- and high fossil-fuel use for electricity and heating or cooling, and between smaller and larger rooms. Also, these are average numbers and will depend on the setup and situation of any specific hotel.

Depending on location, 5–40 kgCO<sub>2</sub>/night over a number of nights amount to emission levels that can be comparable to those of travelling to a meeting location by rail, but are typically dwarfed by flight emissions. In Supplementary Figure 1 we show the contributions of emissions for travel and accommodation for a couple of representative trips with a 6-night stay: a ~800 km trip inside Europe from Leiden/Netherlands to Munich/Germany by train and plane, as well as trips from Australia to China, and South Africa to Canada.

For the intra-Europe train trip the accommodation will make up 55–70% of combined emissions — 20–30% when flying — but for the intercontinental trips it contributes only a few percent. This is, of course, due to the travel emissions being higher by factors of 10–25 in the case of intercontinental trips.

As a rule of thumb, we conclude that a hotel night has a typical GHG emission similar to ~400 km of train travel, or 60–100 km short-distance flying.

## Emission contribution by travel distance

In order to compute the environmental impact depending on the type of travel, we investigate how the number of short-, medium-, and long-haul travel relates to the fraction of GHG emissions associated with each category. For simplicity, we combine long-haul and ultra-long haul travel, since only a very small fraction of travel is longer than 16 hours (0.2%). The distribution is shown in Supplementary Figure 2. Almost two thirds of all trips are short distance travel, which contributes about a fifth to the GHG emissions. Long and ultra-long distance travel, which is often intercontinental, constitutes 21% of all trips, but causes more than 60% of all travel-related emissions. Medium distance trips make up the smallest fraction of all trips (13%), and the related emissions make up almost another 20%.

## Lists of all astronomy conferences and schools in 2019

In our analysis we consider 362 meetings, among which were 307 conferences and 55 schools. We list all countries hosting either conferences, schools, or both in Supplementary Table 1, sorted by continent. Supplementary Tables 2 and 3 list information for each individual conference and school, respectively, for which we could obtain information about the participants’ origin that enabled us to assess the travel-related GHG emissions. Conferences and schools for which we were not able to retrieve the necessary information about participants are listed in Supplementary Tables 4 and 5.

---

<sup>1</sup>Based on emission data by atmosfair gGmbH, Germany, “VDR Standard Part III”, [https://www.atmosfair.de/en/standards/emissions\\_calculation/co2\\_reporting\\_for\\_companies/vdr\\_standard\\_methodology](https://www.atmosfair.de/en/standards/emissions_calculation/co2_reporting_for_companies/vdr_standard_methodology)

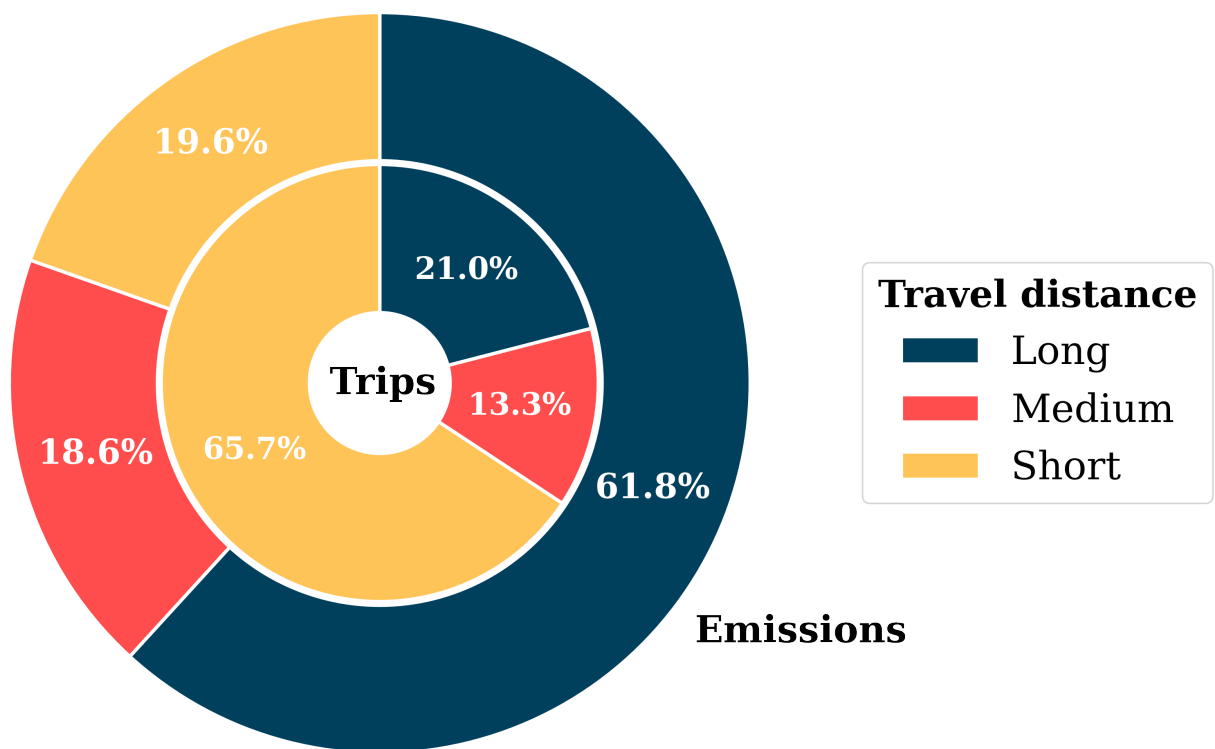

**Supplementary Figure 2:** Nested donut charts displaying the number of conference trips taken and divided by classification (short-, medium-, and long-haul) in the inner ring, versus the total emissions produced for each category in the outer ring. The 'long-haul' classification includes trips with ultra-long distances, which make up 0.2% of all trips and 1.3% of all emissions.

**Supplementary Table 1:** Distribution of conferences and schools over different continents and countries.

| Continent                 | Number of meetings | Country         | Conferences | Schools |
|---------------------------|--------------------|-----------------|-------------|---------|
| Africa                    | 4                  | Ethiopia        | 1           | 0       |
|                           |                    | Nigeria         | 0           | 1       |
|                           |                    | South Africa    | 2           | 0       |
| Asia                      | 61                 | Armenia         | 4           | 1       |
|                           |                    | Azerbaijan      | 1           | 0       |
|                           |                    | China           | 17          | 1       |
|                           |                    | India           | 9           | 8       |
|                           |                    | Iran            | 1           | 0       |
|                           |                    | Israel          | 2           | 0       |
|                           |                    | Japan           | 13          | 0       |
|                           |                    | Kazakhstan      | 1           | 0       |
|                           |                    | Malaysia        | 0           | 1       |
|                           |                    | Russia          | 4           | 2       |
|                           |                    | South Korea     | 1           | 0       |
|                           |                    | Taiwan          | 4           | 1       |
|                           |                    | Thailand        | 0           | 3       |
|                           |                    | Turkey          | 2           | 0       |
|                           |                    | Vietnam         | 1           | 0       |
| Europe                    | 142                | Austria         | 1           | 0       |
|                           |                    | Belgium         | 1           | 0       |
|                           |                    | Bulgaria        | 1           | 0       |
|                           |                    | Czech Republic  | 1           | 0       |
|                           |                    | Denmark         | 1           | 1       |
|                           |                    | Finland         | 2           | 0       |
|                           |                    | France          | 9           | 6       |
|                           |                    | Germany         | 21          | 3       |
|                           |                    | Greece          | 7           | 1       |
|                           |                    | Hungary         | 3           | 0       |
|                           |                    | Iceland         | 1           | 0       |
|                           |                    | Ireland         | 1           | 0       |
|                           |                    | Italy           | 25          | 3       |
|                           |                    | The Netherlands | 21          | 2       |
|                           |                    | Poland          | 1           | 3       |
|                           |                    | Portugal        | 3           | 1       |
|                           |                    | Spain           | 14          | 3       |
|                           |                    | Sweden          | 3           | 0       |
|                           |                    | Switzerland     | 4           | 2       |
|                           |                    | Ukraine         | 1           | 0       |
|                           |                    | United Kingdom  | 22          | 1       |
| North America & Caribbean | 65                 | Canada          | 8           | 0       |
|                           |                    | Cuba            | 1           | 0       |
|                           |                    | Mexico          | 2           | 0       |
|                           |                    | United States   | 63          | 6       |
| Oceania                   | 21                 | Australia       | 18          | 3       |
|                           |                    | New Zealand     | 2           | 0       |
| South America             | 7                  | Argentina       | 2           | 1       |
|                           |                    | Brazil          | 2           | 1       |
|                           |                    | Chile           | 3           | 0       |

**Supplementary Table 2:** List of all 258 conferences with participant data. The number of participants given in parentheses are the amount of local participants, which travelled less than 200 km per round-trip.

| Meeting name                                                                                                                                | Venue                              | Number of participants | Tot. travel emissions (tCO <sub>2</sub> e) | Emission per participant (tCO <sub>2</sub> e) | Distance trav. by train | Note                                        |
|---------------------------------------------------------------------------------------------------------------------------------------------|------------------------------------|------------------------|--------------------------------------------|-----------------------------------------------|-------------------------|---------------------------------------------|
| Africa                                                                                                                                      |                                    |                        |                                            |                                               |                         |                                             |
| Cosmology on Safari                                                                                                                         | KwaZulu-Natal, South Africa        | 76 (12)                | 175.9                                      | 2.30                                          | < 300 km                |                                             |
| Modeling Meerkats: Comparing galaxy formation simulations to MeerKAT surveys                                                                | Kruger National Park, South Africa | 22 (0)                 | 37.61                                      | 1.71                                          | < 300 km                |                                             |
| IAU Symposium 356: Nuclear activity in galaxies                                                                                             | Addis Ababa, Ethiopia              | 180 (20)               | 301.28                                     | 1.67                                          | < 300 km                | One origin not back-traceable               |
| Asia                                                                                                                                        |                                    |                        |                                            |                                               |                         |                                             |
| 5th China-Chile Bi-lateral Astro meeting                                                                                                    | Kunming, China                     | 76 (10)                | 186.63                                     | 2.46                                          | < 700 km                |                                             |
| PERC International Symposium on Dust & Parent bodies (IDP 2019)                                                                             | Tokyo, Japan                       | 35 (15)                | 34.32                                      | 0.98                                          | < 700 km                |                                             |
| The Metrewavelength Sky - II: Celebrating the 90 <sup>th</sup> year of Govind Swarup and the 1st year of the upgraded GMRT                  | Pune, India                        | 187 (69)               | 220.03                                     | 1.18                                          | < 500 km                |                                             |
| Cosmic Lab                                                                                                                                  | Narashino, Japan                   | 17 (8)                 | 9.16                                       | 0.54                                          | < 700 km                |                                             |
| Search for life, from Early Earth to Exoplanets                                                                                             | Quy Nhon, Vietnam                  | 49 (2)                 | 131.54                                     | 2.68                                          | < 300 km                |                                             |
| Extremely big Eyes on the early Universe                                                                                                    | Kashiwa, Japan                     | 78 (22)                | 87.52                                      | 1.12                                          | < 500 km                |                                             |
| The 1st Donglu Astrophysics Forum The era of large-scale sky surveys: Near field cosmology and time domain science                          | Kunming, China                     | 121 (36)               | 55.30                                      | 0.46                                          | < 1000 km               |                                             |
| VHE Phenomena Around Supermassive Black Holes                                                                                               | Yerevan, Armenia                   | 47 (3)                 | 65.63                                      | 1.40                                          | < 300 km                |                                             |
| The 9th International Workshop on Occultation and Eclipse (IWOE9)                                                                           | Canakkale, Turkey                  | 40 (8)                 | 16.29                                      | 0.41                                          | < 1000 km               |                                             |
| The correlated Universe                                                                                                                     | Seogwipo, South Korea              | 38 (0)                 | 42.65                                      | 1.12                                          | < 100 km                |                                             |
| Tal Alexander workshop: Dynamics and accretion near massive black holes                                                                     | Tel Aviv, Israel                   | 63 (49)                | 30.18                                      | 0.48                                          | < 100 km                |                                             |
| Recent progress in relativistic astrophysics                                                                                                | Shanghai, China                    | 88 (4)                 | 112.35                                     | 1.28                                          | < 1000 km               |                                             |
| International Pulsar Timing Array Meeting - 2019                                                                                            | Pune, India                        | 94 (13)                | 220.88                                     | 2.35                                          | < 700 km                |                                             |
| Exploring the Energetic Universe 2019                                                                                                       | Astana, Kazakhstan                 | 16 (4)                 | 20.95                                      | 1.31                                          | < 300 km                |                                             |
| Future Science with Multi-Wavelength Data: North Ecliptic Pole Meeting 2019                                                                 | Hsinchu, Taiwan                    | 45 (20)                | 32.37                                      | 0.72                                          | < 300 km                |                                             |
| IAU Symposium 353: Galactic Dynamics in the Era of Large Surveys                                                                            | Shanghai, China                    | 81 (9)                 | 219.91                                     | 2.71                                          | < 1000 km               | Participants estimated from programme       |
| Cosmic Dust                                                                                                                                 | Narashino, Japan                   | 57 (14)                | 76.51                                      | 1.34                                          | < 700 km                |                                             |
| From AGN to starburst                                                                                                                       | Guiyang, China                     | 107 (3)                | 155.07                                     | 1.45                                          | < 700 km                |                                             |
| Gravity meets Plasma Workshop                                                                                                               | Kunming, China                     | 44 (0)                 | 59.88                                      | 1.36                                          | < 1000 km               |                                             |
| Dynamics of asteroids, TNOS & natural satellites with Gaia data                                                                             | Antalya, Turkey                    | 29 (12)                | 25.58                                      | 0.88                                          | < 300 km                |                                             |
| Active galaxies and quasars                                                                                                                 | Byurakan, Armenia                  | 22 (15)                | 3.52                                       | 0.16                                          | < 300 km                |                                             |
| KIAA Forum on Gas in Galaxies "Multiple-phase Interstellar medium: Probing the Activities and Power Engines from Local to Distant Universe" | Beijing, China                     | 100 (41)               | 111.44                                     | 1.11                                          | < 1000 km               |                                             |
| IAU South West & Asian regional workshop                                                                                                    | Byurakan, Armenia                  | 37 (16)                | 11.90                                      | 0.32                                          | < 300 km                |                                             |
| Compact white dwarf binaries                                                                                                                | Yerevan, Armenia                   | 64 (3)                 | 135.63                                     | 2.12                                          | < 300 km                |                                             |
| Challenges and innovations in computational astrophysics                                                                                    | Saint Petersburg, Russia           | 102 (3)                | 84.40                                      | 0.83                                          | < 700 km                |                                             |
| Physics of Stars and Planets: Atmospheres, Activity, Magnetic fields                                                                        | Shamakh, Azerbaijan                | 111 (42)               | 43.35                                      | 0.39                                          | < 300 km                |                                             |
| Mapping Central regions of AGN                                                                                                              | Shanghai, China                    | 122 (4)                | 233.36                                     | 1.91                                          | < 1000 km               |                                             |
| Multi-messenger astrophysics in gravitational wave era                                                                                      | Kyoto, Japan                       | 165 (28)               | 259.62                                     | 1.57                                          | < 700 km                |                                             |
| Diversity of the local Universe                                                                                                             | Nizhnij Arkhyz, Russia             | 82 (23)                | 78.26                                      | 0.95                                          | < 500 km                |                                             |
| The UX Ori type stars and related topics                                                                                                    | Saint Petersburg, Russia           | 59 (13)                | 47.79                                      | 0.81                                          | < 300 km                |                                             |
| Second Workshop on Numerical Modeling in MHD and Plasma Physics: Methods, Tools, and Outcomes                                               | Moscow, Russia                     | 29 (12)                | 17.82                                      | 0.61                                          | < 500 km                |                                             |
| The Milky Way 2019: LAMOST and Other Leading Surveys                                                                                        | Yichang, China                     | 110 (3)                | 85.72                                      | 0.78                                          | < 1000 km               |                                             |
| New Horizons in Galactic Center Astronomy and Beyond                                                                                        | Yokohama, Japan                    | 136 (37)               | 230.37                                     | 1.69                                          | < 700 km                |                                             |
| Cosmic Evolution of Quasars: from the First Light to Local Relics                                                                           | Beijing, China                     | 112 (28)               | 144.23                                     | 1.29                                          | < 1000 km               |                                             |
| Gamma-ray Bursts in the Gravitational Wave Era 2019                                                                                         | Yokohama, Japan                    | 161 (51)               | 272.47                                     | 1.69                                          | < 700 km                |                                             |
| TMT Science Forum                                                                                                                           | Xiamen Island, China               | 113 (9)                | 160.35                                     | 1.42                                          | < 1000 km               | Origin for some participants not clear      |
| 4th COSPAR Symposium: Small Satellites for Sustainable Science and Development                                                              | Herzliya, Israel                   | 258 (63)               | 434.16                                     | 1.68                                          | < 300 km                |                                             |
| 1st Shanghai assembly on cosmology & galaxy                                                                                                 | Shanghai, China                    | 100 (26)               | 111.15                                     | 1.11                                          | < 1000 km               |                                             |
| Science with the Submillimeter Array: Present and Future                                                                                    | Taipei, Taiwan                     | 108 (51)               | 118.65                                     | 1.10                                          | < 500 km                |                                             |
| JCMt Users                                                                                                                                  | Taipei, Taiwan                     | 87 (40)                | 74.72                                      | 0.86                                          | < 300 km                |                                             |
| Astronomy for equity, diversity and inclusion                                                                                               | Tokyo, Japan                       | 121 (16)               | 289.1                                      | 2.39                                          | < 700 km                |                                             |
| International Conference on Modeling, Machine Learning and Astronomy                                                                        | Bangalore, India                   | 150 (20)               | 71.03                                      | 0.47                                          | < 700 km                | Cities for origin of participants estimated |
| Planet formation workshop                                                                                                                   | Tokyo, Japan                       | 88 (36)                | 71.02                                      | 0.81                                          | < 700 km                |                                             |
| International conference on Gravitation & Cosmology                                                                                         | Punjab, India                      | 196 (1)                | 141.75                                     | 0.72                                          | < 500 km                |                                             |
| Young Astronomers' Meet 2019 at Kodaikanal Solar Observatory                                                                                | Kodaikanal, India                  | 57 (0)                 | 21.26                                      | 0.37                                          | < 700 km                |                                             |
| Modern Engineering Trends in Astronomy - 2019(META-2019)                                                                                    | Bangalore, India                   | 193 (107)              | 25.14                                      | 0.13                                          | < 700 km                |                                             |
| Multi-wavelength Astronomy: Three years of AstroSat observations                                                                            | Bangalore, India                   | 84 (50)                | 12.96                                      | 0.15                                          | < 300 km                |                                             |
| International Symposium on Extra - Solar Planets                                                                                            | Bangalore, India                   | 20 (5)                 | 19.98                                      | 1.00                                          | < 300 km                |                                             |
| 2019 ASROC Annual Meeting                                                                                                                   | Taichung, Taiwan                   | 176 (84)               | 11.23                                      | 0.06                                          | < 500 km                |                                             |

Table 2 continued.

| Meeting name                                                                                              | Venue                      | Number of participants | Tot. travel emissions (tCO <sub>2</sub> e) | Emission per participant (tCO <sub>2</sub> e) | Distance trav. by train | Note                                            |
|-----------------------------------------------------------------------------------------------------------|----------------------------|------------------------|--------------------------------------------|-----------------------------------------------|-------------------------|-------------------------------------------------|
| Europe                                                                                                    |                            |                        |                                            |                                               |                         |                                                 |
| The Supernova-Supernova Remnant Connection                                                                | London, UK                 | 16 (4)                 | 3.64                                       | 0.23                                          | < 300 km                | Only origin countries were known                |
| Spectroscopy with SOFIA: new results & future opportunities                                               | Kreuth, Germany            | 59 (2)                 | 39.14                                      | 0.66                                          | < 500 km                |                                                 |
| Monsters of the Universe: The Most Extreme Star Factories                                                 | Leiden, Netherlands        | 36 (0)                 | 28.31                                      | 0.79                                          | < 500 km                |                                                 |
| Nucleosynthesis for a Life: Symposium in honour of Prof. Roland Diehl                                     | Garching, Germany          | 60 (50)                | 3.69                                       | 0.06                                          | < 500 km                |                                                 |
| 12th INTEGRAL conference                                                                                  | Geneva, Switzerland        | 166 (11)               | 115.14                                     | 0.69                                          | < 500 km                |                                                 |
| Formation of Stars and Massive clusters in Dwarf Galaxies over Cosmic Time                                | Leiden, Netherlands        | 45 (5)                 | 44.54                                      | 0.99                                          | < 500 km                | Only origin continents were known               |
| Large survey with small telescopes                                                                        | Bamberg, Germany           | 79 (13)                | 46.18                                      | 0.58                                          | < 500 km                |                                                 |
| 20 years of FORS                                                                                          | Garching, Germany          | 12 (2)                 | 9.12                                       | 0.76                                          | < 500 km                |                                                 |
| Extreme Precision in Radial Velocity IV                                                                   | Grindelwald, Switzerland   | 121 (0)                | 196.05                                     | 1.62                                          | < 300 km                |                                                 |
| Galaxy Evolution in the Cosmic Web                                                                        | Leiden, Netherlands        | 27 (3)                 | 28.38                                      | 1.05                                          | < 500 km                |                                                 |
| The New Era of Multi-Messenger Astrophysics                                                               | Groningen, Netherlands     | 152 (28)               | 113.44                                     | 0.75                                          | < 500 km                | flights from UK, 500km rule for other countries |
| Turbulence & magnetic fields                                                                              | Helsinki, Finland          | 60 (8)                 | 49.93                                      | 0.83                                          | < 300 km                |                                                 |
| SKA General Science Meeting                                                                               | Macclesfield, UK           | 270 (64)               | 323.51                                     | 1.20                                          | < 300 km                |                                                 |
| ESLAB symposium: the Gaia universe                                                                        | Noordwijk, The Netherlands | 142 (21)               | 67.15                                      | 0.47                                          | < 300 km                |                                                 |
| Laboratory Astrophysics                                                                                   | Cambridge, UK              | 172 (17)               | 163.95                                     | 0.95                                          | < 300 km                |                                                 |
| Delving into the neutron star crust (ICONS)                                                               | Amsterdam, Netherlands     | 38 (9)                 | 47.29                                      | 1.24                                          | < 500 km                |                                                 |
| PHAROS: multimessenger physics & neutron stars                                                            | Barcelona, Spain           | 176 (12)               | 123.52                                     | 0.70                                          | < 500 km                |                                                 |
| Metals in Galaxies, Near and Far: Looking Ahead                                                           | Leiden, Netherlands        | 47 (3)                 | 51.67                                      | 1.10                                          | custom                  |                                                 |
| Preparing for 4MOST                                                                                       | Garching, Germany          | 114 (27)               | 60.13                                      | 0.53                                          | < 500 km                |                                                 |
| 1st CTA Symposium                                                                                         | Bologna, Italy             | 275 (44)               | 249.32                                     | 0.91                                          | < 500 km                |                                                 |
| ExoComets: Understanding the Composition of Planetary Building Blocks                                     | Leiden, Netherlands        | 56 (10)                | 52.85                                      | 0.94                                          | < 700 km                |                                                 |
| Herschel 10 years after launch                                                                            | Madrid, Spain              | 69 (28)                | 34.95                                      | 0.51                                          | < 500 km                |                                                 |
| Multi-messenger astro with SKA                                                                            | Aveiro, Portugal           | 65 (20)                | 53.80                                      | 0.83                                          | < 500 km                |                                                 |
| Meeting of Italian Astronomical Society                                                                   | Rome, Italy                | 145 (58)               | 14.40                                      | 0.10                                          | < 500 km                |                                                 |
| Exploring the Infrared Universe                                                                           | Heraklion, Greece          | 164 (4)                | 271.48                                     | 1.66                                          | < 300 km                |                                                 |
| Multi-spin galaxies                                                                                       | Asiago, Italy              | 32 (8)                 | 30.41                                      | 0.95                                          | < 300 km                | Only origin countries were known                |
| Workshop on Polarization in Protoplanetary Disks and Jets                                                 | Sant Cugat, Spain          | 58 (7)                 | 82.27                                      | 1.42                                          | < 500 km                |                                                 |
| Star clusters: from the MilkyWay to the Early Universe                                                    | Bologna, Italy             | 204 (18)               | 308.42                                     | 1.51                                          | < 500 km                |                                                 |
| From Interstellar medium to large scale structures                                                        | Stockholm, Sweden          | 73 (10)                | 71.29                                      | 0.98                                          | < 500 km                |                                                 |
| Supernova remnants                                                                                        | Chania, Greece             | 193 (4)                | 401.31                                     | 2.08                                          | < 300 km                |                                                 |
| What matter(s) between galaxies: unraveling the knots in the Cosmic Web                                   | Abbazia di Spineto, Italy  | 73 (0)                 | 121.05                                     | 1.66                                          | < 500 km                |                                                 |
| Linking the Milky Way and Nearby Galaxies: The ISM and Star Formation from Cold Cores to Kpc Scales       | Helsinki, Finland          | 99 (6)                 | 165.1                                      | 1.67                                          | < 300 km                |                                                 |
| Planetary Dynamics 2019                                                                                   | Heidelberg, Germany        | 67 (19)                | 62.01                                      | 0.93                                          | < 500 km                |                                                 |
| Partially ionised plasmas in astrophysics                                                                 | Palma de Mallorca, Spain   | 53 (8)                 | 57.00                                      | 1.08                                          | < 300 km                |                                                 |
| IAU Symposium 352: Uncovering early galaxy evolution in the ALMA and JWST era                             | Viana do Castelo, Portugal | 172 (6)                | 312.88                                     | 1.82                                          | < 300 km                |                                                 |
| Joint conference of sub-regional EU astro committee                                                       | Sofia, Bulgaria            | 56 (12)                | 4.38                                       | 0.08                                          | < 500 km                |                                                 |
| Zooming in on Star Formation                                                                              | Nafplio, Greece            | 116 (3)                | 174.47                                     | 1.50                                          | < 300 km                |                                                 |
| New perspectives on galactic magnetism                                                                    | Newcastle upon Tyne, UK    | 61 (6)                 | 72.37                                      | 1.19                                          | < 300 km                |                                                 |
| Astrophysics of hot plasma in extended X-ray sources                                                      | Madrid, Spain              | 78 (6)                 | 110.34                                     | 1.41                                          | < 500 km                |                                                 |
| 5th workshop of SCAR AAA, Astronomy and Astrophysics from Antarctica                                      | Courmayeur, Italy          | 38 (0)                 | 73.93                                      | 1.95                                          | < 1000 km               |                                                 |
| The cosmic web                                                                                            | Edinburgh, UK              | 80 (14)                | 78.95                                      | 0.99                                          | < 500 km                |                                                 |
| From Stars to Planets II - Connecting our understanding of star and planet formation                      | Gothenburg, Sweden         | 161 (14)               | 185.98                                     | 1.16                                          | < 300 km                | Only origin countries were known                |
| Starry                                                                                                    | Leeds, UK                  | 64 (7)                 | 65.81                                      | 1.03                                          | < 300 km                |                                                 |
| 9th meeting on hot subdwarfs                                                                              | Hendaye, France            | 60 (0)                 | 77.38                                      | 1.29                                          | < 500 km                |                                                 |
| Astrochemistry: from nanometers to megaparsecs                                                            | Gothenburg, Sweden         | 79 (19)                | 65.02                                      | 0.82                                          | < 500 km                |                                                 |
| The new era of multi-messenger astrophysics                                                               | Groningen, Netherlands     | 149 (28)               | 110.01                                     | 0.74                                          | < 300 km                |                                                 |
| Ringberg Conference on Star-Planet connection                                                             | Kreuth, Germany            | 49 (0)                 | 30.74                                      | 0.63                                          | < 700 km                |                                                 |
| RAS National Astronomy Meeting 2019                                                                       | Lancaster, UK              | 526 (121)              | 78.23                                      | 0.15                                          | < 300 km                |                                                 |
| Alpine Cosmology Workshop 2019 (ACW19)                                                                    | La Berarde, France         | 20 (1)                 | 6.54                                       | 0.33                                          | < 500 km                |                                                 |
| From winds to jets: the role of outflows in compacts binaries                                             | Amsterdam, Netherlands     | 55 (15)                | 45.10                                      | 0.82                                          | < 500 km                |                                                 |
| The Beginnings and Ends of Double White Dwarfs                                                            | Copenhagen, Denmark        | 72 (21)                | 95.43                                      | 1.33                                          | < 500 km                |                                                 |
| 14th International Conference on Numerical Modeling of Space Plasma Flows (ASTRONUM-2019)                 | Paris, France              | 82 (7)                 | 136.14                                     | 1.66                                          | < 300 km                |                                                 |
| 14th hellenic astronomical conference                                                                     | Volos, Greece              | 139 (2)                | 56.57                                      | 0.41                                          | < 300 km                |                                                 |
| Tracing Cosmic Evolution with Clusters of Galaxies IV                                                     | Sesto, Italy               | 255 (1)                | 359.21                                     | 1.41                                          | < 300 km                |                                                 |
| Turbulence, Structure Formation and Accretion in Protoplanetary Disks: Theory, Observation and Experiment | Kreuth, Germany            | 60 (5)                 | 61.83                                      | 1.03                                          | < 500 km                |                                                 |

Table 2 continued.

| Meeting name                                                                                                                               | Venue                               | Number of participants | Tot. travel emissions (tCO <sub>2</sub> e) | Emission per participant (tCO <sub>2</sub> e) | Distance trav. by train | Note                                                                                  |
|--------------------------------------------------------------------------------------------------------------------------------------------|-------------------------------------|------------------------|--------------------------------------------|-----------------------------------------------|-------------------------|---------------------------------------------------------------------------------------|
| IAU Symposium 355: The Realm of the Low Surface Brightness Universe                                                                        | La Laguna, Spain                    | 120 (15)               | 201.05                                     | 1.68                                          | < 100 km                | Only origin countries were known                                                      |
| High Energy phenomena in relativist outflows                                                                                               | Barcelona, Spain                    | 97 (13)                | 106.30                                     | 1.10                                          | < 500 km                |                                                                                       |
| Astronomy in Ukraine: from archaeoastronomy to high-energy astrophysics.                                                                   | Kyiv, Ukraine                       | 71 (45)                | 11.38                                      | 0.16                                          | < 300 km                |                                                                                       |
| XCalibur 2019 – High resolution X-ray spectroscopy as a probe of strong gravity and dark matter: From Hitomi to XRISM and beyond to Athena | Southampton, UK                     | 74 (10)                | 75.32                                      | 1.02                                          | < 300 km                |                                                                                       |
| A centenary of astrophysical jets                                                                                                          | Cheshire, UK                        | 119 (17)               | 128.8                                      | 1.08                                          | < 300 km                |                                                                                       |
| Understanding cosmological observations                                                                                                    | Benasque, Spain                     | 65 (0)                 | 73.32                                      | 1.13                                          | < 500 km                |                                                                                       |
| Nine Billion Years of Neutral Gas Evolution                                                                                                | Garching, Germany                   | 84 (15)                | 151.08                                     | 1.80                                          | < 500 km                |                                                                                       |
| Small galaxies, cosmic questions                                                                                                           | Durham, UK                          | 131 (20)               | 188.91                                     | 1.44                                          | < 300 km                |                                                                                       |
| Quasars in crisis                                                                                                                          | Edinburgh, UK                       | 69 (10)                | 86.40                                      | 1.25                                          | < 300 km                |                                                                                       |
| Improving Image Fidelity on Astronomical Data: Radio Interferometer and Single-Dish Data Combination                                       | Leiden, Netherlands                 | 44 (7)                 | 59.55                                      | 1.35                                          | < 500 km                |                                                                                       |
| Extreme solar systems IV                                                                                                                   | Reykjavik, Iceland                  | 583 (2)                | 928.25                                     | 1.59                                          | < 100 km                |                                                                                       |
| Stars and their Variability, Observed from Space                                                                                           | Vienna, Austria                     | 256 (30)               | 249.95                                     | 0.98                                          | < 500 km                |                                                                                       |
| Stars on the Run II                                                                                                                        | Potsdam, Germany                    | 70 (16)                | 43.03                                      | 0.61                                          | < 500 km                | Participant list ~ 40% incomplete                                                     |
| Astro Hack Week 2019                                                                                                                       | Cambridge, UK                       | 34 (4)                 | 47.65                                      | 1.40                                          | < 300 km                |                                                                                       |
| 49th Young European Radio Astronomers Conference                                                                                           | Dublin, Ireland                     | 34 (7)                 | 13.57                                      | 0.40                                          | < 300 km                |                                                                                       |
| Matera Oscura                                                                                                                              | Matera, Italy                       | 139 (2)                | 145.76                                     | 1.05                                          | < 500 km                |                                                                                       |
| Physics & chemistry of interstellar medium                                                                                                 | Avignon, France                     | 123 (0)                | 135.71                                     | 1.10                                          | < 500 km                |                                                                                       |
| Views on interstellar medium in galaxies with ALMA                                                                                         | Bologna, Italy                      | 116 (23)               | 105.43                                     | 0.91                                          | < 500 km                |                                                                                       |
| Variable Galactic Gamma-Ray Sources (VGGRS) V                                                                                              | Barcelona, Spain                    | 45 (8)                 | 51.01                                      | 1.13                                          | < 300 km                |                                                                                       |
| Astrophysics with GW detections                                                                                                            | Warsaw, Poland                      | 58 (22)                | 40.89                                      | 0.70                                          | < 500 km                |                                                                                       |
| Universe of Binaries, Binaries in the Universe                                                                                             | Telc, Czech Republic                | 88 (7)                 | 91.54                                      | 1.04                                          | < 300 km                |                                                                                       |
| X-ray astronomy 2019                                                                                                                       | Bologna, Italy                      | 315 (35)               | 324.60                                     | 1.03                                          | < 500 km                |                                                                                       |
| A synoptic view of the magellanic clouds                                                                                                   | Garching, Germany                   | 104 (15)               | 165.45                                     | 1.59                                          | < 500 km                |                                                                                       |
| Stars as probes of first-star nucleosynthesis                                                                                              | Geneva, Switzerland                 | 78 (18)                | 113.94                                     | 1.46                                          | < 700 km                |                                                                                       |
| Extremely big eyes on the early universe                                                                                                   | Rome, Italy                         | 96 (21)                | 70.32                                      | 0.73                                          | < 500 km                | Abstract book used for affiliations                                                   |
| Nuclear Physics in Astrophysics IX                                                                                                         | Frankfurt, Germany                  | 139 (51)               | 92.44                                      | 0.67                                          | < 500 km                |                                                                                       |
| IAU Astronomy Education Conference: Bridging Research & Practice                                                                           | Garching, Germany                   | 114 (4)                | 150.45                                     | 1.32                                          | < 500 km                |                                                                                       |
| From Gas to stars                                                                                                                          | York, UK                            | 82 (17)                | 81.30                                      | 1.00                                          | < 500 km                | Only origin countries were known                                                      |
| The 3C extragalactic radio sky                                                                                                             | Torino, Italy                       | 98 (17)                | 106.36                                     | 1.09                                          | < 500 km                |                                                                                       |
| The extragalactic explosive universe                                                                                                       | Garching, Germany                   | 102 (14)               | 88.14                                      | 0.86                                          | < 300 km                |                                                                                       |
| Meeting of Astronomische Gesellschaft 2019                                                                                                 | Stuttgart, Germany                  | 219 (64)               | 48.25                                      | 0.22                                          | < 700 km                |                                                                                       |
| Cosmology: the end of the beginning. Future prospects in cosmology, large scale structure and galaxy formation                             | Cambridge, UK                       | 153 (56)               | 141.18                                     | 0.92                                          | < 300 km                |                                                                                       |
| Statistics to the Stars and Back: Convincing Inference Across the Interdisciplinary Gap                                                    | Leiden, Netherlands                 | 32 (25)                | 0.81                                       | 0.03                                          | custom                  |                                                                                       |
| Rotation periods of cool stars                                                                                                             | Potsdam, Germany                    | 54 (14)                | 45.65                                      | 0.85                                          | < 500 km                | Data available on how many trains and planes were taken                               |
| Crete III - Through dark lanes to new stars: Celebrating the career of Prof. Charles Lada                                                  | Crete, Greece                       | 93 (3)                 | 183.23                                     | 1.97                                          | no train                |                                                                                       |
| Bonn Gravity 2019                                                                                                                          | Bonn, Germany                       | 74 (26)                | 61.93                                      | 0.84                                          | < 500 km                |                                                                                       |
| The time machine factory                                                                                                                   | Torino, Italy                       | 82 (29)                | 39.78                                      | 0.49                                          | < 500 km                |                                                                                       |
| YAGN19 - Young Astronomers on Galactic Nuclei                                                                                              | La Laguna, Spain                    | 29 (5)                 | 32.84                                      | 1.13                                          | < 300 km                |                                                                                       |
| The legacy of the gaia-eso survey                                                                                                          | Firenze, Italy                      | 89 (18)                | 75.00                                      | 0.84                                          | < 500 km                |                                                                                       |
| 38th International Meteor Conference                                                                                                       | Bollmannsruh, Germany               | 99 (11)                | 39.07                                      | 0.39                                          | < 500 km                |                                                                                       |
| ADASS                                                                                                                                      | Groningen, Netherlands              | 350 (67)               | 438.54                                     | 1.25                                          | < 500 km                |                                                                                       |
| Untangle the skein with Scarlet (LSST)                                                                                                     | Rome, Italy                         | 37 (6)                 | 9.17                                       | 0.25                                          | < 300 km                |                                                                                       |
| Cosmic Ray anisotropy workshop                                                                                                             | Rome, Italy                         | 58 (16)                | 53.11                                      | 0.92                                          | < 500 km                | Participants based on statement of organisers, assuming most participants are from UK |
| RAS Specialist Discussion Meeting: Common envelope evolution and post-common-envelope systems                                              | London, UK                          | 40 (13)                | 6.41                                       | 0.16                                          | < 300 km                |                                                                                       |
| SKA-VLBI Key Science workshop                                                                                                              | Cheshire, UK                        | 65 (19)                | 86.59                                      | 1.33                                          | < 500 km                |                                                                                       |
| ALMA2019: science results and cross-facility synergies                                                                                     | Cagliari, Italy                     | 235 (3)                | 433.38                                     | 1.84                                          | no train                |                                                                                       |
| Historical Supernovae, Novae and Other Transient Events                                                                                    | Leiden, Netherlands                 | 30 (5)                 | 31.26                                      | 1.04                                          | < 700 km                |                                                                                       |
| The Future of X-ray Timing                                                                                                                 | Amsterdam, Netherlands              | 123 (27)               | 122.49                                     | 1.00                                          | < 500 km                |                                                                                       |
| First Galaxies, First Structures                                                                                                           | Paris, France                       | 60 (15)                | 57.17                                      | 0.95                                          | < 500 km                |                                                                                       |
| EMU international meeting                                                                                                                  | Catania, Italy                      | 27 (8)                 | 40.26                                      | 1.49                                          | < 500 km                |                                                                                       |
| Revolutionary Spectroscopy of Today as a Springboard to Webb                                                                               | Leiden, Netherlands                 | 54 (4)                 | 86.66                                      | 1.60                                          | < 700 km                |                                                                                       |
| Voyage 2050 workshop - Shaping the European Space Agency's space science plan for 2035-2050                                                | Madrid, Spain                       | 262 (1)                | 159.43                                     | 0.61                                          | < 300 km                | Only origin continents were known                                                     |
| Scintillometry 2019                                                                                                                        | Bonn, Germany                       | 63 (14)                | 90.16                                      | 1.43                                          | < 500 km                |                                                                                       |
| First Spanish Meeting on Galaxy Clusters                                                                                                   | Madrid, Spain                       | 41 (15)                | 16.16                                      | 0.39                                          | < 500 km                |                                                                                       |
| Lithium in the Universe: to Be or not to Be?                                                                                               | Rome, Italy                         | 84 (6)                 | 104.84                                     | 1.25                                          | < 500 km                |                                                                                       |
| The art of measuring galaxy physical properties                                                                                            | Milano, Italy                       | 133 (8)                | 182.68                                     | 1.37                                          | < 500 km                |                                                                                       |
| PHYSICS and ASTROPHYSICS of COSMIC RAYS                                                                                                    | Saint Michel l'Observatoire, France | 40 (5)                 | 15.02                                      | 0.38                                          | < 500 km                |                                                                                       |
| WorkPlaNS II: Workshop for Planetary Nebula observations                                                                                   | Leiden, Netherlands                 | 50 (3)                 | 72.02                                      | 1.44                                          | < 500 km                |                                                                                       |
| The Origins of Black Hole Mergers and Gravitational                                                                                        | Leiden, Netherlands                 | 35 (9)                 | 51.40                                      | 1.47                                          | < 500 km                |                                                                                       |

Table 2 continued. <sup>†</sup>Origin cities used for US states are state capitols, except for the following states, for which we took the cities given in parentheses instead: Alabama (Tuscaloosa), Arizona (Tucson, Flagstaff), California (Los Angeles, San Diego, San Francisco), Connecticut (New Haven), Illinois (Chicago), Maryland (Baltimore), Michigan (Lansing, Ann Arbor), Minnesota (Minneapolis), Missouri (Saint Louis), New Mexico (Albuquerque, Socorro), New York (Albany, Ithaca, New York City, Rochester), Pennsylvania (Philadelphia, State College), South Carolina (Clemson, Columbia), Texas (Austin, Houston, Dallas), Virginia (Charlottesville, Lynchburg), Washington (Bellingham, Pullman, Seattle), and West Virginia (Morgantown). For states with more than two listed cities we divided the number of participants equally.

| Meeting name                                                                                            | Venue                    | Number of participants | Tot. travel emissions (tCO <sub>2</sub> e) | Emission per participant (tCO <sub>2</sub> e) | Distance trav. by train | Note                                                               |
|---------------------------------------------------------------------------------------------------------|--------------------------|------------------------|--------------------------------------------|-----------------------------------------------|-------------------------|--------------------------------------------------------------------|
| 10th OPTICON Gaia Science Alerts Workshop                                                               | Catania, Italy           | 54 (5)                 | 37.67                                      | 0.70                                          | < 500 km                |                                                                    |
| 5ème atelier PLATO/France: Synergies PLATO/ARIEL                                                        | Bordeaux, France         | 44 (5)                 | 2.22                                       | 0.05                                          | < 700 km                |                                                                    |
| AO4ASTRO                                                                                                | Marseille, France        | 62 (23)                | 28.81                                      | 0.46                                          | < 500 km                |                                                                    |
| TRAPPIST-1: Towards the Comparative Study of Temperate Terrestrial Worlds                               | Liège, Belgium           | 90 (23)                | 82.95                                      | 0.92                                          | < 300 km                |                                                                    |
| Interstellar Exploration                                                                                | Noordwijk, Netherlands   | 30 (16)                | 0.43                                       | 0.01                                          | custom                  | Data included how many trains and planes were taken                |
| Exoclimes V                                                                                             | Oxford, UK               | 139 (24)               | 192.2                                      | 1.38                                          | < 300 km                |                                                                    |
| European Planetary Science Congress - AAS Division Planetary Science Joint Meeting                      | Geneva, Switzerland      | 1730 (52)              | 2341.71                                    | 1.35                                          | < 500 km                | Only origin countries were known                                   |
| Wavefront sensing in the VLT/ELT era                                                                    | Firenze, Italy           | 81 (24)                | 33.42                                      | 0.41                                          | < 500 km                |                                                                    |
| MW-Gaia WG3 Workshop: Exoplanets in the era of Gaia                                                     | Porto, Portugal          | 36 (10)                | 16.32                                      | 0.45                                          | < 500 km                |                                                                    |
| EAS Meeting 2019                                                                                        | Lyon, France             | 1462 (0)               | 1034.80                                    | 0.71                                          | < 500 km                |                                                                    |
| North & Central America                                                                                 |                          |                        |                                            |                                               |                         |                                                                    |
| 233rd AAS meeting                                                                                       | Seattle, WA, USA         | 3396 (118)             | 3461.97                                    | 1.02                                          | < 300 km                | Only origin country and US states <sup>†</sup> were known          |
| Testing Gravity 2019                                                                                    | Vancouver, Canada        | 117 (26)               | 159.70                                     | 1.36                                          | < 300 km                |                                                                    |
| 23rd International Microlensing Conference                                                              | Pasadena, CA, USA        | 82 (16)                | 133.90                                     | 1.63                                          | < 300 km                | Data for 2019 conference not available, used 2017 participant list |
| Extremely big eyes on the early universe                                                                | Los Angeles, CA, USA     | 70 (17)                | 54.74                                      | 0.78                                          | < 300 km                |                                                                    |
| Massively multiplexed spectroscopy with MSE                                                             | Tucson, AZ, USA          | 93 (11)                | 122.9                                      | 1.32                                          | < 300 km                |                                                                    |
| Into the Starlight: The End of the Cosmic Dark Ages                                                     | Aspen, CO, USA           | 61 (0)                 | 98.08                                      | 1.61                                          | < 300 km                |                                                                    |
| Dusting the Universe                                                                                    | Tucson, AZ, USA          | 82 (7)                 | 125.24                                     | 1.53                                          | < 300 km                | Origin for one participant not retrievable                         |
| Kepler & K2 Science Conference V                                                                        | Glendale, CA, USA        | 283 (67)               | 331.27                                     | 1.17                                          | < 300 km                |                                                                    |
| HEAD 17th Divisional Meeting                                                                            | Monterey, CA, USA        | 362 (25)               | 444.7                                      | 1.23                                          | < 300 km                |                                                                    |
| CHARA 2019                                                                                              | Flagstaff, AZ, USA       | 47 (15)                | 36.20                                      | 0.77                                          | < 500 km                |                                                                    |
| r-process sources in the universe                                                                       | Tempe, AZ, USA           | 37 (6)                 | 38.82                                      | 1.05                                          | no train                |                                                                    |
| New quests in stellar astrophysics IV                                                                   | Puerto Vallarta, Mexico  | 109 (0)                | 141.48                                     | 1.30                                          | < 300 km                |                                                                    |
| The Landscape of Space Astrophysics in the 2020s and Beyond                                             | Potomac, MD, USA         | 84 (47)                | 30.84                                      | 0.37                                          | < 100 km                | Participants estimated from programme                              |
| Better Stars, Better Planets: Exploiting the Stellar-Exoplanetary Synergy                               | Santa Barbara, CA, USA   | 69 (6)                 | 98.78                                      | 1.43                                          | < 300 km                |                                                                    |
| The Deaths and Afterlives of Stars                                                                      | Baltimore, MD, USA       | 143 (28)               | 161.64                                     | 1.13                                          | < 300 km                |                                                                    |
| The Future of Canadian Radio Astronomy                                                                  | Penticton, Canada        | 45 (12)                | 19.76                                      | 0.44                                          | < 300 km                |                                                                    |
| Stars 2019                                                                                              | Havana, Cuba             | 53 (14)                | 81.75                                      | 1.54                                          | < 300 km                |                                                                    |
| New Horizons in planetary systems                                                                       | Victoria, Canada         | 144 (21)               | 192.95                                     | 1.34                                          | < 500 km                |                                                                    |
| The New Era of Gravitational-Wave Physics and Astrophysics                                              | Santa Barbara, CA, USA   | 69 (6)                 | 100.02                                     | 1.45                                          | < 300 km                |                                                                    |
| Canada-France-Hawaii Telescope 12th Users' Meeting                                                      | Montreal, Canada         | 130 (38)               | 142.8                                      | 1.10                                          | < 300 km                |                                                                    |
| F.O.E. Fifty-One Erg Supernova Conference                                                               | Raleigh, NC, USA         | 116 (16)               | 196.38                                     | 1.69                                          | < 300 km                |                                                                    |
| Memorial Symposium to honor Riccardo Giacconi                                                           | Washington DC, USA       | 106 (44)               | 67.80                                      | 0.64                                          | custom                  | data with means of transportation were provided                    |
| 234th AAS meeting                                                                                       | St. Louis, MO, USA       | 753 (71)               | 511.97                                     | 0.68                                          | < 300 km                | Only origin country and US states <sup>†</sup> were known          |
| 2019 Canadian Astronomical Society Annual Meeting                                                       | Montreal, Canada         | 302 (85)               | 184.19                                     | 0.61                                          | < 300 km                |                                                                    |
| Exploring the Galaxy and the Local Group with WFIRST                                                    | Pasadena, CA, USA        | 79 (45)                | 38.69                                      | 0.49                                          | < 300 km                |                                                                    |
| Gordon Conference on Origins of Solar Systems                                                           | South Hadley, MA, USA    | 121 (4)                | 136.50                                     | 1.13                                          | < 300 km                |                                                                    |
| Astroinformatics 2019                                                                                   | Pasadena, CA, USA        | 59 (32)                | 61.60                                      | 1.04                                          | < 300 km                |                                                                    |
| SDSS-IV/V Collaboration meeting                                                                         | Ensenada, Mexico         | 142 (37)               | 164.02                                     | 1.16                                          | < 300 km                |                                                                    |
| Radio/Millimeter Astrophysical Frontiers next decade                                                    | Charlottesville, VA, USA | 115 (41)               | 61.41                                      | 0.53                                          | < 300 km                |                                                                    |
| Kavli Summer Program In Astrophysics 2019: Machine Learning in the era of large astronomical surveys    | Santa Barbara, CA, USA   | 35 (0)                 | 60.84                                      | 1.74                                          | < 300 km                |                                                                    |
| Space climate 7                                                                                         | Canton Orford, Canada    | 76 (0)                 | 119.58                                     | 1.57                                          | < 500 km                |                                                                    |
| TASC5/KASC12 workshop                                                                                   | Cambridge, MA, USA       | 118 (13)               | 204.24                                     | 1.73                                          | < 300 km                |                                                                    |
| TESS Science Conference I                                                                               | Cambridge, MA, USA       | 282 (92)               | 316.03                                     | 1.12                                          | < 300 km                |                                                                    |
| Long Wavelength Array Users Meeting                                                                     | Albuquerque, NM, USA     | 42 (14)                | 15.01                                      | 0.36                                          | < 300 km                |                                                                    |
| Multiscale Phenomena in Plasma Astrophysics                                                             | Santa Barbara, CA, USA   | 75 (1)                 | 134.14                                     | 1.79                                          | < 300 km                | Participants estimated from conference picture                     |
| LSST 2019 Project and Community Workshop                                                                | Tucson, AZ, USA          | 300 (106)              | 241.34                                     | 0.80                                          | no train                |                                                                    |
| VISTA Variables in Via Lactea (VVV) 10th Science meeting.                                               | Hilo, HI, USA            | 25 (9)                 | 53.28                                      | 2.13                                          | < 100 km                |                                                                    |
| Hot-wiring the transient universe VI                                                                    | Evanston, IL, USA        | 93 (19)                | 99.82                                      | 1.07                                          | < 300 km                |                                                                    |
| Non-Standard Cosmology Probes                                                                           | Aspen, CO, USA           | 40 (0)                 | 76.32                                      | 1.91                                          | no train                |                                                                    |
| Connecting Micro and Macro Scales: Acceleration, Reconnection, and Dissipation in Astrophysical Plasmas | Santa Barbara, CA, USA   | 76 (5)                 | 129.00                                     | 1.70                                          | < 300 km                |                                                                    |
| The Cosmic Baryon Cycle: Impact on Galaxy Evolution                                                     | Carlsbad, CA, USA        | 103 (12)               | 137.16                                     | 1.33                                          | < 300 km                |                                                                    |
| Midwest workshop on Supernovae and transients                                                           | Columbus, OH, USA        | 67 (24)                | 17.81                                      | 0.27                                          | < 300 km                |                                                                    |

Table 2 continued.

| Meeting name                                                                                                              | Venue                     | Number of participants | Tot. travel emissions (tCO <sub>2</sub> e) | Emission per participant (tCO <sub>2</sub> e) | Distance trav. by train | Note                                                             |
|---------------------------------------------------------------------------------------------------------------------------|---------------------------|------------------------|--------------------------------------------|-----------------------------------------------|-------------------------|------------------------------------------------------------------|
| Managing Follow-up Observations in the Era of ZTF and LSST                                                                | Pasadena, CA, USA         | 51 (11)                | 83.01                                      | 1.63                                          | < 300 km                |                                                                  |
| Cosmic controversies                                                                                                      | Chicago, IL, USA          | 281 (98)               | 204.87                                     | 0.73                                          | < 300 km                |                                                                  |
| Warm Ionized Medium in Galaxies Workshop                                                                                  | Green Bank, WV, USA       | 45 (6)                 | 29.43                                      | 0.65                                          | < 100 km                |                                                                  |
| The RR Lyrae and Cepheid Conference 2019: Frontiers of Classical Pulsators - Theory and Observations                      | Cloudcroft, NM, USA       | 75 (0)                 | 165.59                                     | 2.21                                          | no train                |                                                                  |
| IAU Symposium 357: White Dwarfs as probes of fundamental physics and tracers of planetary, stellar and galactic evolution | Hilo, HI, USA             | 93 (9)                 | 250.40                                     | 2.69                                          | no train                |                                                                  |
| Rocky Exoplanets in the era of JWST                                                                                       | Greenbelt, MD, USA        | 125 (70)               | 58.66                                      | 0.47                                          | < 300 km                | Participants taken from picture, their origin from contributions |
| The New Faces of Black Holes, 2019 JSI Workshop                                                                           | Annapolis, MD, USA        | 70 (21)                | 45.05                                      | 0.64                                          | < 300 km                |                                                                  |
| Subaru Telescope 20th Anniversary - Optical & Infrared Astronomy for the Next Decade                                      | Waikoloa, HI, USA         | 240 (35)               | 453.88                                     | 1.89                                          | < 100 km                |                                                                  |
| Universality: Turbulence across vast scales                                                                               | New York City, NY, USA    | 67 (30)                | 43.99                                      | 0.66                                          | < 300 km                |                                                                  |
| Twenty Years of Science with Chandra                                                                                      | Boston, MA, USA           | 285 (154)              | 172.85                                     | 0.61                                          | < 300 km                |                                                                  |
| Science at Low Frequencies VI                                                                                             | Tempe, AZ, USA            | 132 (17)               | 260.86                                     | 1.98                                          | < 300 km                |                                                                  |
| Keck Wide-Field Imager Science Workshop                                                                                   | Pasadena, CA, USA         | 41 (13)                | 61.41                                      | 1.50                                          | < 300 km                |                                                                  |
| TESS Data Workshop                                                                                                        | Baltimore, MD, USA        | 80 (10)                | 72.87                                      | 0.91                                          | < 100 km                | No data on origin cities                                         |
| Telluric Line Hack Week                                                                                                   | New York City, NY, USA    | 44 (3)                 | 43.62                                      | 0.99                                          | < 300 km                |                                                                  |
| Chesapeake Bay Area Exoplanet Meeting                                                                                     | Baltimore, MD, USA        | 60 (55)                | 0.66                                       | 0.01                                          | < 300 km                |                                                                  |
| Planet-Star Connections in the Era of TESS and Gaia                                                                       | Santa Barbara, CA, USA    | 70 (8)                 | 114.14                                     | 1.63                                          | < 100 km                | No data on origin cities                                         |
| 2019 Mid-American Regional Astrophysics Conference (MARAC)                                                                | Atchison, USA             | 50 (17)                | 6.30                                       | 0.13                                          | < 300 km                |                                                                  |
| Oceania                                                                                                                   |                           |                        |                                            |                                               |                         |                                                                  |
| 12th PHISCC workshop                                                                                                      | Perth, Australia          | 80 (24)                | 167.17                                     | 2.09                                          | < 300 km                | Uncertainty for city origin within Australia                     |
| Linking galaxies from the epoch of initial star formation to today                                                        | Sydney, Australia         | 162 (57)               | 437.36                                     | 2.70                                          | < 500 km                |                                                                  |
| The life and death of starforming regions                                                                                 | Perth, Australia          | 91 (16)                | 306.4                                      | 3.37                                          | < 300 km                |                                                                  |
| LSST@Asia                                                                                                                 | Sydney, Australia         | 102 (9)                | 257.60                                     | 2.53                                          | < 300 km                |                                                                  |
| Barefoot reionization                                                                                                     | Fitzroy Island, Australia | 85 (0)                 | 278.66                                     | 3.28                                          | < 300 km                |                                                                  |
| Great Barriers in Planet Formation                                                                                        | Palm Cove, Australia      | 115 (0)                | 461.27                                     | 4.01                                          | no train                |                                                                  |
| Astronomical Data Archives                                                                                                | Sydney, Australia         | 42 (9)                 | 86.80                                      | 2.07                                          | < 300 km                |                                                                  |
| New Zealand Starlight Conference                                                                                          | Lake Tekapo, New Zealand  | 132 (11)               | 142.37                                     | 1.08                                          | < 300 km                |                                                                  |
| Exploiting Large Radio and mm Surveys to understand the ISM                                                               | Kingscliff, Australia     | 22 (0)                 | 14.12                                      | 0.64                                          | < 300 km                |                                                                  |
| New Zealand Square Kilometre Array Forum                                                                                  | Auckland, New Zealand     | 48 (24)                | 28.11                                      | 0.59                                          | no train                |                                                                  |
| ACAMAR5 - Healesville                                                                                                     | Melbourne, Australia      | 82 (18)                | 139.89                                     | 1.71                                          | no train                |                                                                  |
| Dynamical Models of Observed Galaxies                                                                                     | Sydney, Australia         | 25 (15)                | 11.81                                      | 0.47                                          | no train                |                                                                  |
| ASA ASM                                                                                                                   | Brisbane, Australia       | 233 (25)               | 147.41                                     | 0.63                                          | no train                |                                                                  |
| Astronomical Data Archives                                                                                                | Sydney, Australia         | 42 (12)                | 88.48                                      | 2.11                                          | no train                |                                                                  |
| Stars in Melbourne Workshop                                                                                               | Melbourne, Australia      | 37 (19)                | 12.67                                      | 0.34                                          | no train                |                                                                  |
| MAVIS Workshop                                                                                                            | Sydney, Australia         | 19 (12)                | 3.22                                       | 0.17                                          | no train                |                                                                  |
| ASTRO 3D annual retreat                                                                                                   | Ballarat, Australia       | 95 (0)                 | 54.26                                      | 0.57                                          | < 300 km                |                                                                  |
| ASTRO 3D science meeting                                                                                                  | Sydney, Australia         | 86 (23)                | 56.34                                      | 0.66                                          | no train                |                                                                  |
| South America                                                                                                             |                           |                        |                                            |                                               |                         |                                                                  |
| The La Silla Observatory - inauguration to future                                                                         | La Serena, Chile          | 73 (7)                 | 168.06                                     | 2.30                                          | < 500 km                |                                                                  |
| 9th Friends of Friends Meeting                                                                                            | Cordoba, Argentina        | 133 (84)               | 84.80                                      | 0.64                                          | < 500 km                |                                                                  |
| Workshop de Infraestructura Astronómica argentina                                                                         | Cordoba, Argentina        | 83 (46)                | 16.14                                      | 0.19                                          | < 300 km                |                                                                  |
| Precision spectroscopy workshop                                                                                           | Sao Paulo, Brazil         | 43 (27)                | 14.54                                      | 0.34                                          | < 500 km                |                                                                  |
| IAU meeting: Regional Latin-American                                                                                      | Antofagasta, Chile        | 330 (29)               | 247.57                                     | 0.75                                          | < 500 km                |                                                                  |

**Supplementary Table 3:** List of all 42 schools with participant data. The number of participants given in parentheses are the amount of local participants, which travelled less than 200 km per round-trip.

| Meeting name                                                                            | Venue                            | Number of participants | Tot. travel emissions (tCO <sub>2</sub> e) | Emission per participant (tCO <sub>2</sub> e) | Distance trav. by train | Note                                              |
|-----------------------------------------------------------------------------------------|----------------------------------|------------------------|--------------------------------------------|-----------------------------------------------|-------------------------|---------------------------------------------------|
| Africa                                                                                  |                                  |                        |                                            |                                               |                         |                                                   |
| West African International Summer School for Young Astronomers                          | Abuja, Nigeria                   | 70 (11)                | 32.65                                      | 0.47                                          | < 300 km                | Estimated origin cities for students from Nigeria |
| Asia                                                                                    |                                  |                        |                                            |                                               |                         |                                                   |
| Cosmogly – The Next Decade                                                              | Bangalore, India                 | 43 (7)                 | 48.03                                      | 1.12                                          | < 700 km                | Only country of origin known                      |
| The 1st Thai-CTA workshop on Astroparticle Physics                                      | Chiang Mai, Thailand             | 74 (8)                 | 46.00                                      | 0.62                                          | < 300 km                |                                                   |
| Astrowin19 - Winter School on Astronomy                                                 | Hyderabad, India                 | 64 (11)                | 33.67                                      | 0.53                                          | < 500 km                |                                                   |
| A COSPAR capacity building workshop                                                     | Punjab, India                    | 35 (1)                 | 22.49                                      | 0.64                                          | < 300 km                |                                                   |
| NARIT-EACOA Summer Workshop on Astrostatistics & Astroinformatics                       | Chiang Mei, Thailand             | 54 (7)                 | 36.77                                      | 0.68                                          | < 300 km                |                                                   |
| IFAS5 - Astronomy summer school - Spectroscopy & Spectrographs                          | Pune, India                      | 31 (14)                | 13.79                                      | 0.44                                          | < 300 km                |                                                   |
| Regional summer school on space sciences                                                | Byurakan, Armenia                | 23 (15)                | 5.43                                       | 0.24                                          | < 300 km                |                                                   |
| 1st Malaysian VLBI Workshop                                                             | Kuala Lumpur, Malaysia           | 54 (29)                | 28.37                                      | 0.53                                          | < 300 km                |                                                   |
| APCTP School/Workshop on Gravitational-Wave Cosmology                                   | Taipei, Taiwan                   | 100 (35)               | 81.84                                      | 0.82                                          | < 300 km                |                                                   |
| Solar Physics Summer School at Raman Science Center, Leh                                | Leh, India                       | 50 (0)                 | 56.78                                      | 1.14                                          | < 300 km                |                                                   |
| 42nd International school for Young Astronomers                                         | Kunming, China                   | 64 (23)                | 44.41                                      | 0.69                                          | < 1000 km               |                                                   |
| 8th IIST Astronomy and Astrophysics School - 2019                                       | Thiruvananthapuram, India        | 47 (1)                 | 17.08                                      | 0.36                                          | < 500 km                |                                                   |
| Europe                                                                                  |                                  |                        |                                            |                                               |                         |                                                   |
| The Milky Way in the Gaia Era                                                           | Saas Fee, Switzerland            | 38 (0)                 | 48.68                                      | 1.28                                          | < 500 km                | Only country of origin known                      |
| Gravitational wave open data workshop                                                   | Paris, France                    | 54 (18)                | 30.50                                      | 0.56                                          | < 500 km                |                                                   |
| Multiple approaches to plasma physics                                                   | Les Houches, France              | 70 (1)                 | 57.28                                      | 0.82                                          | < 700 km                |                                                   |
| Advanced school on exoplanetary science                                                 | Salerno, Italy                   | 86 (5)                 | 72.80                                      | 0.85                                          | < 500 km                |                                                   |
| Cosmic explosions 2019                                                                  | Cargese, France                  | 54 (0)                 | 51.85                                      | 0.96                                          | < 100 km                |                                                   |
| SPACE ASTROMETRY FOR ASTROPHYSICS                                                       | L'Aquila, Italy                  | 55 (1)                 | 70.70                                      | 1.29                                          | < 500 km                |                                                   |
| Cracow school of Theoretical physics                                                    | Zakopane, Poland                 | 69 (44)                | 26.43                                      | 0.38                                          | < 500 km                |                                                   |
| Torun Astrophysics, Spectroscopy and Quantum Chemistry school                           | Torun, Poland                    | 60 (19)                | 25.20                                      | 0.42                                          | < 500 km                |                                                   |
| Artificial Intelligence in Astronomy                                                    | Garching, Germany                | 122 (28)               | 101.80                                     | 0.83                                          | < 500 km                |                                                   |
| Summer school on protoplanetary disks                                                   | Copenhagen, Denmark              | 53 (15)                | 42.62                                      | 0.80                                          | < 500 km                |                                                   |
| IRAM 30m summer school                                                                  | Granada, Spain                   | 43 (4)                 | 39.43                                      | 0.92                                          | < 500 km                |                                                   |
| Heidelberg summer school: Instrumentation for Ground-based Optical & Infrared Astronomy | Heidelberg, Germany              | 51 (10)                | 41.13                                      | 0.81                                          | < 500 km                |                                                   |
| Torun summer school: Polarimetry as diagnostic tool in astronomy                        | Torun, Poland                    | 34 (9)                 | 13.04                                      | 0.38                                          | < 500 km                |                                                   |
| School of Statistics for Astrophysics 2019: Variability and Time Series Analysis        | Autrans, France                  | 20 (5)                 | 2.71                                       | 0.14                                          | < 500 km                |                                                   |
| 1st IAA-CSIC Severo Ochoa School on Statistics, Data Mining and Machine Learning        | Granada, Spain                   | 45 (20)                | 25.89                                      | 0.58                                          | < 500 km                |                                                   |
| NYRIA workshop 2019                                                                     | Lisbon, Portugal                 | 19 (3)                 | 15.14                                      | 0.80                                          | < 300 km                |                                                   |
| CNRS thematic school of astroparticle physics                                           | Manosque, France                 | 40 (5)                 | 15.02                                      | 0.38                                          | < 500 km                |                                                   |
| Astroparticle School ECAP                                                               | Obertrubach, Germany             | 41 (1)                 | 9.62                                       | 0.23                                          | < 700 km                |                                                   |
| North & Central America                                                                 |                                  |                        |                                            |                                               |                         |                                                   |
| Multiscale Modeling of Astrophysical and Space Plasmas                                  | New York City, USA               | 41 (1)                 | 57.61                                      | 1.41                                          | < 300 km                | Only country of origin known                      |
| 2019 Sagan Exoplanet Summer Workshop                                                    | Pasadena, California, USA        | 35 (12)                | 31.24                                      | 0.89                                          | < 100 km                |                                                   |
| GROWTH astronomy school                                                                 | San Diego, USA                   | 149 (62)               | 102.15                                     | 0.69                                          | < 300 km                |                                                   |
| CfAO Summer school on adaptive optics                                                   | Santa Cruz, California, USA      | 48 (9)                 | 60.10                                      | 1.25                                          | < 300 km                |                                                   |
| Summer school on statistics in Astronomy                                                | State College, Pennsylvania, USA | 50 (10)                | 51.38                                      | 1.03                                          | < 500 km                |                                                   |
| Fermi Summer School                                                                     | Lewes, Delaware, USA             | 28 (0)                 | 37.48                                      | 1.34                                          | < 300 km                |                                                   |
| Oceania                                                                                 |                                  |                        |                                            |                                               |                         |                                                   |
| ASTRO 3D East Coast writing retreat                                                     | Sydney, Australia                | 19 (15)                | 0.93                                       | 0.05                                          | no train                | Remote attendants excluded                        |
| ASTRO 3D proposal writing workshop                                                      | Canberra, Australia              | 21 (14)                | 1.13                                       | 0.05                                          | no train                |                                                   |
| CASS Radio Astronomy School 2019                                                        | Narrabri, Australia              | 57 (1)                 | 33.53                                      | 0.59                                          | < 500 km                |                                                   |
| South America                                                                           |                                  |                        |                                            |                                               |                         |                                                   |
| First Light                                                                             | Sao Paulo, Brazil                | 117 (26)               | 198.4                                      | 1.98                                          | < 500 km                |                                                   |
| La plata international school                                                           | La Plata, Argentina              | 57 (24)                | 54.2                                       | 0.95                                          | < 300 km                |                                                   |

**Supplementary Table 4:** List of conferences lacking data on the origin cities, countries or continents for the participants. If not noted otherwise, the average participant number for each continent was used depending on the conference location. We use the continent-specific mean emissions per participant to estimate the total amount of travel-related GHG emission for each meeting (see Table 1).

| Name                                                                                                                                | Venue                       | Number of participants | Tot. travel emissions (tCO <sub>2</sub> e) | Note                                                                 |
|-------------------------------------------------------------------------------------------------------------------------------------|-----------------------------|------------------------|--------------------------------------------|----------------------------------------------------------------------|
| Asia                                                                                                                                |                             |                        |                                            |                                                                      |
| Baryons in Galaxies and Beyond                                                                                                      | Teheran, Iran               | 80                     | 88.0                                       | Participant number estimated from picture                            |
| Gamma-Ray Bursts and Related Astrophysics in Multi-Messenger Era                                                                    | Nanjing, China              | 91                     | 100.1                                      |                                                                      |
| 14th International Astronomical Consortium for High Energy Calibration meeting                                                      | Kanagawa, Japan             | 58                     | 63.8                                       | Participant number estimated from programme and picture              |
| Atomic Structure and Oscillator Strengths for astrophysical and fusion plasma research                                              | Shanghai, China             | 91                     | 100.1                                      |                                                                      |
| 15th International Symposium on Origin of Matter and Evolution of Galaxies                                                          | Kyoto, Japan                | 91                     | 100.1                                      |                                                                      |
| Astrophysical Dynamics                                                                                                              | Shanghai, China             | 91                     | 100.1                                      |                                                                      |
| Progenitors of Type Ia supernovae                                                                                                   | Lijiang, China              | 100                    | 110.0                                      | Organisers report ~ 100 participants                                 |
| Galaxy Angular Momentum Alignment 2019                                                                                              | Shanghai, China             | 91                     | 100.1                                      |                                                                      |
| In the Spirit of Lyot 2019                                                                                                          | Tokyo, Japan                | 91                     | 100.1                                      |                                                                      |
| Planet2/RESCEU Symposium: From Protoplanetary Disks through Planetary System Architecture to Planetary Atmospheres and Habitability | Okinawa, Japan              | 91                     | 100.1                                      |                                                                      |
| IRIS 10 @ IIA and CHRIST                                                                                                            | Bangalore, India            | 91                     | 100.1                                      |                                                                      |
| Europe                                                                                                                              |                             |                        |                                            |                                                                      |
| Thermal Models in Planetary Science III                                                                                             | Budapest, Hungary           | 45                     | 45.0                                       | Participant number estimated from programme                          |
| Enabling LISA Science Exploitation                                                                                                  | Leiden, Netherlands         | 40                     | 40.0                                       | Participant number based on typical size of Lorentz-Center workshops |
| MOSAIC 2019: Science and Surveys with the ELT Multi-Object Spectrograph                                                             | Heidelberg, Germany         | 50                     | 50.0                                       | Participant number guessed                                           |
| UK Exoplanet Community Meeting                                                                                                      | London, UK                  | 103                    | 103.0                                      |                                                                      |
| Electron-Capture-Initiated Stellar Collapse                                                                                         | Leiden, Netherlands         | 40                     | 40.0                                       | Participant number based on typical size of Lorentz-Center workshops |
| Light in the suburbs: structure and chemo-dynamics of galaxy halos                                                                  | Sexten, Italy               | 103                    | 103.0                                      |                                                                      |
| Supermassive Black Holes: environment and evolution                                                                                 | Corfu Town, Greece          | 103                    | 103.0                                      |                                                                      |
| Stellar Hydro Days V                                                                                                                | Exeter, UK                  | 103                    | 103.0                                      |                                                                      |
| Feedback and its Role in Galaxy Formation                                                                                           | Spetses, Greece             | 100                    | 100.0                                      | Organisers report ~ 100 participants                                 |
| CosmoCruise2019: From the Early to the Late Universe                                                                                | Venice, Italy               | 103                    | 103.0                                      |                                                                      |
| Understanding the nearby star forming Universe with JWST                                                                            | Courmayeur, Italy           | 50                     | 50.0                                       | Participant number estimated from picture                            |
| Irish National Astronomy Meeting 2019                                                                                               | Armagh, UK                  | 103                    | 103.0                                      |                                                                      |
| The Pleiades and friends: stellar associations in the Gaia era                                                                      | A Coruña, Spain             | 103                    | 103.0                                      |                                                                      |
| 6th Workshop on Robotic Autonomous Observatories                                                                                    | Torremolinos, Spain         | 103                    | 103.0                                      |                                                                      |
| Interaction of Stars with their Environment 2019                                                                                    | Budapest, Hungary           | 30                     | 30.0                                       | Participant number guessed                                           |
| PLATO atmospheres workshop                                                                                                          | Berlin, Germany             | 40                     | 40.0                                       | Participant number guessed                                           |
| Plato Workshop - Single, Shallow, and Strange transits                                                                              | Warwick, UK                 | 103                    | 103.0                                      |                                                                      |
| Exoplanet Vision 2050 workshop                                                                                                      | Budapest, Hungary           | 70                     | 70.0                                       | Max. participants ~ 70                                               |
| South East Exoplanet Meetings                                                                                                       | London, UK                  | 30                     | 30.0                                       | Participant number guessed                                           |
| North & Central America                                                                                                             |                             |                        |                                            |                                                                      |
| Midwest Magnetic Fields Workshop 2019                                                                                               | Madison, WI, USA            | 40                     | 48.0                                       | Participant number estimated from programme                          |
| MMT Observatory 40th Anniversary Symposium                                                                                          | Tucson, AZ, USA             | 110                    | 132.0                                      |                                                                      |
| 50th Annual Division on Dynamic Astronomy Meeting                                                                                   | Boulder, CO, USA            | 110                    | 132.0                                      |                                                                      |
| Stellar Magnetism: A Celebration of the Contributions of J.D. Landstreet                                                            | London, Canada              | 40                     | 48.0                                       | Participant number estimated from proceedings                        |
| Python in Astronomy 2019                                                                                                            | Baltimore, MD, USA          | 50                     | 60.0                                       | Participant number estimated from picture                            |
| Understanding Dust 30 Years After CCM                                                                                               | Boulder, CO, USA            | 50                     | 60.0                                       | Participant number guessed                                           |
| Astrophysics in the LIGO/Virgo Era                                                                                                  | Aspen, CO, USA              | 20                     | 24.0                                       | Participant number guessed                                           |
| 258th ACS National Meeting, Symposium on Water in the Universe                                                                      | San Diego, CA, USA          | 45                     | 54.0                                       | Participant number guessed                                           |
| SciCoder Workshop                                                                                                                   | Kampala, HI, USA            | 20                     | 24.0                                       | Participant number guessed                                           |
| 2019 AAVSO 108th Annual Meeting                                                                                                     | Las Cruces, NM, USA         | 80                     | 96.0                                       | Participant number guessed                                           |
| NASA Hubble Fellows Program Symposium                                                                                               | Washington DC, USA          | 24                     | 28.8                                       | Participant number guessed                                           |
| Brown Dwarf to Exoplanet Connection III                                                                                             | Newark, DE, USA             | 45                     | 54.0                                       | Participant number guessed from two previous meetings                |
| AO4ELT6 Adaptive Optics for Extremely Large Telescope                                                                               | Quebec, Canada              | 210                    | 252.0                                      | Participant number estimated from picture                            |
| Emerging Researchers in Exoplanet Science                                                                                           | Ithaca, NY, USA             | 60                     | 72.0                                       | Participant number guessed                                           |
| WFIRST Exoplanet Imaging Data Challenge                                                                                             | New York City, NY, USA      | 20                     | 24.0                                       | Participant number guessed                                           |
| Oceania                                                                                                                             |                             |                        |                                            |                                                                      |
| ANITA workshop and astroinformatics 2019                                                                                            | Melbourne, Australia        | 80                     | 26.5                                       | Participant number estimated from picture                            |
| ASTRO 3D writing retreat                                                                                                            | Coogee, NSW, Australia      | 19                     | 30.4                                       | Participant number guessed                                           |
| South America                                                                                                                       |                             |                        |                                            |                                                                      |
| II Workshop Chemical Abundances in Gaseous Nebulae: Open Problems in Nebular Astrophysics                                           | Sao Jose dos Campos, Brazil | 60                     | 72.0                                       | Participant number estimated from picture                            |
| IAU Symposium 354 - Solar and Stellar Magnetic Fields: Origins and Manifestations                                                   | Copiapo, Chile              | 70                     | 84.0                                       | Participant number estimated from proceedings                        |

**Supplementary Table 5:** List of schools lacking data on the origin cities, countries or continents for the participants. If not noted otherwise, the average participant number for each continent was used depending on the conference location. We use the continent-specific mean emissions per participant to estimate the total amount of travel-related GHG emissions for each meeting (see Table 1 in the main paper manuscript).

| Name                                                                                 | Venue                                                 | Number of Participants | Tot. travel emissions (tCO <sub>2</sub> e) | Note                                                            |
|--------------------------------------------------------------------------------------|-------------------------------------------------------|------------------------|--------------------------------------------|-----------------------------------------------------------------|
| Asia                                                                                 |                                                       |                        |                                            |                                                                 |
| IIA Summer Programme                                                                 | Kodaikanal, India                                     | 38                     | 24.70                                      | Number of participants known, assumed mainly Indian origin      |
| Kodaikanal winter school on solar physics                                            | Kodaikanal, India                                     | 40                     | 26.00                                      | Maximum number of participants known                            |
| NARIT-IOGS Optical Design Summer School 2019                                         | Chiang Mai, Thailand                                  | 25                     | 16.25                                      | Used participant numbers from similar school in 2016            |
| "BASIS" Foundation Summer School 2019: Evolution of Galaxies and Stars               | Sotchi, Russia                                        | 25                     | 16.25                                      | Participant number guessed from programme                       |
| Particles and Cosmology: the 16th Baksan School on Astroparticle Physics             | Baksan Valley, Kabardino-Balkaria, Russian Federation | 25                     | 16.25                                      | Participant number estimated from picture                       |
| Europe                                                                               |                                                       |                        |                                            |                                                                 |
| Ecole Evry Schatzman du PNPS - Interactions étoile - planètes                        | France                                                | 54                     | 37.26                                      |                                                                 |
| Computational Fluid Dynamics in Astrophysics                                         | La Laguna, Tenerife, Spain                            | 65                     | 44.85                                      | Participant number estimated from picture                       |
| XIII Tonale Winter School on Cosmology                                               | Tonale, Italy                                         | 45                     | 31.05                                      | Organisers reported participant numbers and continent of origin |
| Light Anti-Nuclei as a Probe for New Physics                                         | Netherlands                                           | 29                     | 37.26                                      | Participant number listed in meeting report                     |
| St Andrews Monte Carlo Radiation Hydrodynamics Summer School                         | St. Andrews, UK                                       | 54                     | 37.26                                      |                                                                 |
| 4th OBSPM/LAM Summer School Galaxy Formation and Evolution in a Cosmological Context | Spetses, Greece                                       | 30                     | 30.70                                      | Maximum number of participants taken from previous school       |
| Advancing Theoretical Astrophysics                                                   | Amsterdam, Netherlands                                | 54                     | 37.26                                      |                                                                 |
| Exoclimes Simulation Platform (ESP) Inaugural Summer School                          | Guarda Val, Switzerland                               | 54                     | 37.26                                      |                                                                 |
